# Supplementary material for: Trusted Hardware Acceleration for Malicious-Secure Function Secret Sharing
Source: arXiv:2610.04818 source file (2026-10-03)
Supplement: Supplementary file 1 [file A_functionalities.tex]

% ==================================================================
% Appendix A: ideal functionalities and the protected-module resource
% Labels defined here: app:func, app:func-circuit, app:func-pir, app:func-module
% ==================================================================
\section{Ideal Functionalities and the Protected-Module Resource}\label{app:func}

This appendix states in full the objects that \cref{fig:func}, \cref{def:security} and \cref{def:leakage} summarize: the circuit functionality $\FC$ (\cref{app:func-circuit}), the PIR functionality $\FPIR$ (\cref{app:func-pir}), and the ideal resource $\mathcal{F}_{\mathsf{T}}$ that represents one protected module under \ProfT (\cref{app:func-module}). The proofs in \cref{app:proof-dpf,app:proof-auth,app:proof-gates,app:proof-pir,app:proof-main} refer to these definitions and to no other trust assumption.

\textbf{Real and ideal executions.}
We use the real/ideal paradigm for static malicious adversaries with abort~\cite{canetti2000security,goldreich2004foundations,hazay2010efficient,lindell2017simulate}. Fix a manifest $\mu$ and a security parameter $\lambda$. In the real execution $\Real_{\Pi,\Adv,\Env}(\lambda)$, an environment $\Env$ chooses the honest inputs, receives the honest outputs, and interacts freely with the adversary $\Adv$. Before the execution starts, $\Adv$ corrupts at most one computing host, that is, the CPU, operating system, driver, runtime, GPU, host memory and network interface of one party $P_c$, $c\in\{0,1\}$. The corrupt host may deviate arbitrarily: it may issue any command to its local instance of $\mathcal{F}_{\mathsf{T}}$, modify, replay, reorder, delay or drop any message or buffer under its control, and stop at any time. The protected modules $T_0,T_1$ are never corrupted; each is represented by one instance of $\mathcal{F}_{\mathsf{T}}$. In the ideal execution $\Ideal_{\mathcal{F},\Sim,\Env}(\lambda)$ with $\mathcal{F}\in\{\FC,\FPIR\}$, honest parties forward their inputs to $\mathcal{F}$ and output whatever it returns, while a simulator $\Sim$ plays the corrupt party and receives only the leakage and the corrupt outputs that $\mathcal{F}$ hands to it. \Cref{def:security} requires, for every PPT $\Adv$, a PPT $\Sim$ such that for every $\Env$
\[
\bigl|\Pr[\Real_{\Pi,\Adv,\Env}(\lambda)=1]-\Pr[\Ideal_{\mathcal{F},\Sim,\Env}(\lambda)=1]\bigr|\le\epsilon ,
\]
where $\epsilon$ is the explicit bound of \cref{thm:main}. Security is with abort: $\Adv$ may prevent honest outputs, and neither fairness nor availability is provided. The statement covers one admitted execution, namely one session with one manifest. Independent sessions use fresh identities, epochs and keys (\cref{sec:proto-setup}); we do not claim universal composability~\cite{canetti2001universally} or security for concurrent sessions that share module state.

\subsection{Circuit Functionality}\label{app:func-circuit}

\textbf{Manifest.}
The public manifest $\mu$ contains the protocol version; the session identities and roles; the field $\Fp$ with $p=2^{61}-1$ and the tag count $t$; the numeric encoding (fixed-point scale, signed encoding, truncation rule, saturation and range behavior, output decoding); the finite circuit $C$ with its gate identifiers, wire identifiers and tensor shapes; the approved public tables and interval coefficients; the authorized recipient of every output; the input interface and validation rules of every input wire; and the public batch schedule. For an input wire $\omega$ we write $\mathsf{In}_\omega$ for its declared interface (canonical encoding, shape and admissible range) and $O_\omega$ for its designated owner. We write $\mathcal{V}$ for the finite set of validity predicates of $\mu$ and $y_1,\dots,y_K$ for the outputs of $C$, where output $y_k$ has the authorized recipient $R_k$. The manifest hash is bound into the session at setup (\cref{sec:proto-setup}), so both modules and both hosts agree on $\mu$ or the session aborts.

\smallskip
\noindent\fbox{\begin{minipage}{\dimexpr\columnwidth-2\fboxsep-2\fboxrule\relax}
\footnotesize
\centerline{\textbf{Functionality} $\FC$}
\vspace{2pt}\hrule\vspace{3pt}
\textbf{Parameters:} public manifest $\mu$ (circuit $C$ over $\Fp$, interfaces $\mathsf{In}_\omega$, predicates $\mathcal{V}$, recipients $R_k$, schedule). \textbf{Parties:} input owners, $P_0,P_1$, recipients; $\Sim$ controls the statically corrupted party.
\begin{enumerate}[leftmargin=*,nosep,label=\arabic*.]
\item \textbf{Inputs.} For every input wire $\omega$: if $O_\omega$ is honest, receive $x_\omega\in\mathsf{In}_\omega$ from $O_\omega$; if $O_\omega$ is corrupted, receive from $\Sim$ any $x^\star_\omega\in\mathsf{In}_\omega$ and set $x_\omega\gets x^\star_\omega$. A malformed or missing input causes abort. Send $(\mathsf{input},\omega)$ and the public metadata of $\omega$ to $\Sim$.
\item \textbf{Validation.} Compute $\mathsf{val}(x)=(V(x))_{V\in\mathcal{V}}$ on the recorded inputs and send it to $\Sim$. If some $V(x)=0$, send $(\mathsf{abort},V)$ to all parties and halt.
\item \textbf{Evaluation.} Compute $(y_1,\dots,y_K)\gets C(x)$ exactly in the finite arithmetic of $\mu$, including every declared comparison, truncation, table lookup and piecewise polynomial.
\item \textbf{Corrupt and public outputs.} Send to $\Sim$ every $y_k$ whose recipient $R_k$ is corrupted and every $y_k$ that $\mu$ declares public.
\item \textbf{Delivery.} At each public interaction boundary of the schedule, $\Sim$ may send $\mathsf{delay}$ or $\mathsf{abort}$. On $\mathsf{abort}$, send $\mathsf{abort}$ to every honest party and halt. Otherwise, when $\Sim$ sends $(\mathsf{deliver},k)$, give $y_k$ to its honest recipient $R_k$.
\end{enumerate}
\end{minipage}}
\smallskip

\textbf{Leakage.}
The leakage of \cref{def:leakage} is the tuple
\[
\Leak(\mu,x)=\bigl(\mu,\ \ell(\mu),\ \mathsf{sched}(\mu),\ \mathsf{pub}(x),\ \mathsf{val}(x)\bigr),
\]
where $\ell(\mu)$ collects the public message lengths, $\mathsf{sched}(\mu)$ the public interaction and batch schedule, $\mathsf{pub}(x)$ the outputs that $\mu$ declares public (the authorized public openings), and $\mathsf{val}(x)$ the validation and abort outcomes. Lengths and schedules are functions of $\mu$ alone. Masked openings such as $d=x-a$, $c=x+r$ or the XOR vector of a LUT gate are not part of $\Leak$: they are uniform and are simulated (\cref{app:proof-main}). DPF keys, raw FSS outputs, challenges, residuals and MAC keys never appear in $\Leak$.

\textbf{Extraction.}
The input of a corrupted owner is whatever the input protocol fixes, namely $x^\star=r+\epsilon$ for the full mask $r$ and the bound masked difference $\epsilon$ of \cref{fig:arith}. $\FC$ accepts any value in the declared interface; it does not model an input that an application hopes the adversary would use.

\textbf{Validity outcomes are leakage.}
When a validity predicate depends on private inputs, its accept or abort bit is revealed. $\FC$ lists this bit explicitly in $\Leak$ so that an input-dependent validity bit cannot be silently excluded from the analysis. Honest input ranges and intermediate numeric bounds should be established statically whenever possible (\cref{sec:arch-field}), which keeps such predicates input independent.

\textbf{Exact finite semantics.}
$\FC$ evaluates the declared finite circuit over $\Fp$. It is neither a real-valued network nor $\Z_{2^{64}}$ arithmetic. The distance between $C$ and an intended floating-point model (polynomial or table approximation error, fixed-point rounding) is an accuracy property of the compiler and is not a security error. A ring-based deployment requires a different functionality and a different authenticated backend (\cref{sec:proto-repr}).

\textbf{Gate implementation is public.}
Whether a nonlinear gate is compiled to a direct protected gate, a small XOR-masked LUT or an interval FSS gate (\cref{sec:proto-direct}) is recorded in $\mu$. All choices implement the same gate of $C$; the choice is part of $\mu$ and therefore of $\Leak$, and it does not change $\FC$.

\textbf{Model provenance.}
By default, model weights are a private input of their owner and may be chosen freely. To bind a pre-approved model, $\mu$ includes a commitment to canonical quantized weight bytes that the client or an independent model authority authorized. The interface $\mathsf{In}_\omega$ of the weight wires then contains only the byte strings that open this commitment, and the protected loader hashes exactly the bytes that it shares. A public architecture hash alone does not authenticate private weights.

\textbf{Clients.}
In the principal inference statement the external client is honest and does not collude with a computing party; we give no guarantee against client and server collusion. A corrupt computing party may still choose its own inputs and may be the authorized recipient of its own outputs.

\subsection{PIR Functionality}\label{app:func-pir}

Let $\delta_D=(\mathsf{id},\mathsf{ver},N,\mathsf{enc},\mathsf{com}_D)$ be the public snapshot descriptor, where $\mathsf{com}_D$ commits to the database identifier, the version, the shape, the record encoding and the ordered record bytes. Let $D=(D[0],\dots,D[N-1])$ be the snapshot that $\mathsf{com}_D$ binds; a second opening of the same commitment is a binding failure and is charged to $\eps{bind}$ in \cref{thm:main}.

\smallskip
\noindent\fbox{\begin{minipage}{\dimexpr\columnwidth-2\fboxsep-2\fboxrule\relax}
\footnotesize
\centerline{\textbf{Functionality} $\FPIR$}
\vspace{2pt}\hrule\vspace{3pt}
\textbf{Parameters:} descriptor $\delta_D$ and the committed snapshot $D$.
\begin{enumerate}[leftmargin=*,nosep,label=\arabic*.]
\item \textbf{Query.} Receive $(\mathsf{query},\alpha)$ from the client. If the request is malformed or $\alpha\notin\{0,\dots,N-1\}$, send $\mathsf{reject}$ to the client and to $\Sim$ and halt. Otherwise send $\delta_D$ and the public lengths and schedule of the query to $\Sim$.
\item \textbf{Retrieval.} Set $y\gets D[\alpha]$; for a multi-field record, $y$ contains every coordinate of $D[\alpha]$.
\item \textbf{Delivery.} $\Sim$ may send $\mathsf{abort}$, and then the client receives $\mathsf{abort}$; otherwise the client receives $y$.
\end{enumerate}
\textbf{Corruption regimes (separate statements).}
\begin{enumerate}[leftmargin=*,nosep,label=(R\arabic*)]
\item \textbf{Malicious server host:} the client is honest and $\Sim$ corrupts at most one server host; $\Sim$ learns nothing beyond Step~1.
\item \textbf{Malicious client:} both server hosts are honest and only the client is corrupted; in Step~1, $\Sim$ chooses $\alpha^\star$ (extraction) and in Step~3 it receives $D[\alpha^\star]$ only.
\end{enumerate}
\end{minipage}}
\smallskip

\textbf{Scope of the two regimes.}
The regimes are not combined: $\FPIR$ is not claimed against a malicious client that colludes with a malicious server host. Regime (R1) is the integrity and query-privacy statement; regime (R2) is the database-privacy statement. The public descriptor $\delta_D$, including the snapshot commitment, is leakage in both regimes.

\textbf{Padding and boundary cases.}
For $N\ge 2$ the protocol pads the snapshot to $2^n$ records with $n=\lceil\log_2 N\rceil$ and authorizes only $\alpha<N$; for $N=1$ it uses a constant-record special case with the same snapshot and release checks (\cref{alg:pir}). Padding is invisible in $\FPIR$ because only $\alpha<N$ is admissible and both the true and the padded length are functions of $\delta_D$.

\textbf{What the statement is not.}
$\FPIR$ is realized under trusted modules. It does not turn untrusted two-server DPF-PIR~\cite{chor1998private,boyle2016function} into symmetric PIR without additional mechanisms. A verifiable-FSS alternative with externally generated keys~\cite{decastro2022vfss} would have to prove client key validity and server-answer integrity separately, and authenticated PIR~\cite{colombo2023apir} targets integrity in a different trust model.

\subsection{Ideal Protected-Module Resource}\label{app:func-module}

The resource $\mathcal{F}_{\mathsf{T}}$ captures the premise of \ProfT: the code, keys, input parser, arithmetic, state transitions, local memory, protected peer channel and approved I/O paths of a module are correct and confidential. There are two instances $\mathcal{F}_{\mathsf{T}}^{(0)}$ and $\mathcal{F}_{\mathsf{T}}^{(1)}$, one per party. Instance $\mathcal{F}_{\mathsf{T}}^{(b)}$ accepts commands from host $b$ and from external endpoints over authenticated confidential channels, and it talks to its peer instance over an ideal protected channel.

\smallskip
\noindent\fbox{\begin{minipage}{\dimexpr\columnwidth-2\fboxsep-2\fboxrule\relax}
\footnotesize
\centerline{\textbf{Resource} $\mathcal{F}_{\mathsf{T}}^{(b)}$\textbf{: state, channel and global rule}}
\vspace{2pt}\hrule\vspace{3pt}
\textbf{State.} Role $b$; session identifier $\mathsf{sid}$; epoch $\mathsf{ep}$; manifest $\mu$; status $\in\{\mathsf{active},\mathsf{poisoned}\}$; a joint random function $R$ shared with the peer instance, which returns an independent uniform string for every new label and the same string to both instances for the same joint label; global MAC keys $\Delta_1,\dots,\Delta_t$ and their additive shares $\Delta_{0,j},\Delta_{1,j}$ (joint draws); a ledger that maps every gate to one of \lstate{NEW}, \lstate{RESERVED}, \lstate{PREPARED}, \lstate{FROZEN}, \lstate{VERIFIED}, \lstate{CONSUMED}, \lstate{RELEASED}, \lstate{ABORTED}; a frozen store; the set of burned randomness identifiers.

\smallskip
\textbf{Peer channel.} Messages between the two instances are delivered privately and unmodified. The adversary learns their lengths and times and may delay or drop them; a missing message leads to abort.

\smallskip
\textbf{Global rule.} Every command first checks that the status is $\mathsf{active}$, that the frame is canonical (length prefixed, field elements below $p$, no truncation, extra bytes or duplicate identifiers) and that $\mu$ allows the requested ledger transition. Any failure executes \cmd{ABORT}. No command authenticates a host-supplied value.
\end{minipage}}
\smallskip

\smallskip
\noindent\fbox{\begin{minipage}{\dimexpr\columnwidth-2\fboxsep-2\fboxrule\relax}
\footnotesize
\centerline{\textbf{Resource} $\mathcal{F}_{\mathsf{T}}^{(b)}$\textbf{: commands (from host $b$ unless noted)}}
\vspace{2pt}\hrule\vspace{3pt}
\begin{enumerate}[leftmargin=*,nosep,label=\arabic*.]
\item \cmd{OPEN_SESSION}: with the peer instance, agree on the ordered identities, roles $0$ and $1$, $\mathsf{sid}$, a fresh $\mathsf{ep}$, the manifest hash, the field and tag parameters and the protocol version, or abort. Return a session capability and $\Delta_{b,1},\dots,\Delta_{b,t}$ to host $b$.
\item \cmd{RESERVE_PREP}$(g,\mathit{ids})$: if $g$ is \lstate{NEW} and $\mathit{ids}$ are unused, burn $\mathit{ids}$ and set \lstate{RESERVED}; draw the preprocessing of $g$ from $R$ (masks, triples with $c=ab$, authenticated bits, internally held FSS material) and share it with \AuthShare{}; set \lstate{PREPARED} and return the tuples of party $b$ once. For an input gate, also send the full mask $r$ to the owner over its confidential channel and bind the owner's $\epsilon$ after comparing it with the peer; for a private output, send the full output mask to the recipient.
\item \cmd{FREEZE_BATCH}$(g,\mathit{bytes},\mathit{dims},\mathit{wires})$: parse canonically; copy the bytes into the frozen store or into immutable AEAD pages bound to sequence numbers, lengths, gate identifiers and a protected root; hash the descriptor and the bytes; set \lstate{FROZEN}; return the handle and the root.
\item \cmd{CHECK_OPEN}$(h)$: with the peer, run \cref{alg:checkopen} on the frozen bytes of handle $h$; on acceptance set \lstate{VERIFIED} and return the authorized opened values; otherwise return one generic failure and execute \cmd{ABORT}.
\item \cmd{EVAL_FSS}$(g,h)$: only for a \lstate{VERIFIED} masked opening bound to $g$ and role $b$; evaluate the bound FSS or direct gate internally, apply the epilogue, set \lstate{CONSUMED} and return the fresh tuple $\authb{y}{b}$.
\item \cmd{VERIFY_MATRIX}$(g,h)$: for operands anchored to authoritative records, run \cref{alg:freivalds} on the frozen candidate; return a verified immutable handle or execute \cmd{ABORT}.
\item \cmd{FINAL_OUTPUT}$(g,R_k)$: only for a \lstate{VERIFIED} output opening; set \lstate{RELEASED} and send the opened value to $R_k$ with a certificate binding $\mathsf{sid}$, $\mathsf{ep}$, $g$, $R_k$, the output hash and the terminal status.
\item \cmd{ABORT} (host or internal): set the status to $\mathsf{poisoned}$ and every open gate to \lstate{ABORTED}; withhold all candidate values and pending responses; draw no further challenge; never return burned identifiers to a free list.
\end{enumerate}
\end{minipage}}
\smallskip

\textbf{Observable trace.}
Besides command outputs, host $b$ observes the timing, lengths and access pattern of the external interface of its module (DMA requests, peer traffic, spill pages). The model stipulates a trace simulator: a PPT algorithm that produces this trace from the command sequence, $\mu$, the public lengths and the accept or abort outcomes, with distinguishing advantage at most $\eps{trace}$. This is an assumption on the implementation (constant-time engines, fixed-pattern scans, data-independent spill schedules), not a theorem, and it is listed as a deployment obligation in \cref{tab:obligations}.

\textbf{Error terms.}
$\eps{setup}$ covers the realization of \cmd{OPEN_SESSION} by attestation and authenticated key establishment; $\eps{channel}$ covers the realization of the peer channel and of the client channels; $\eps{prf}$ covers the replacement of the joint random function $R$ by a PRF or KDF with length-prefixed labels; $\eps{bind}$ covers collisions and forgeries of manifests, snapshots, frozen roots, certificates and session freshness; $\eps{trace}$ covers the trace simulator. The correctness of protected code, state and arithmetic is a premise of the resource. It is not a probability that we estimate or measure.

\textbf{Outside the resource.}
Physical probing, fault injection, power and electromagnetic analysis, microarchitectural or speculative-execution bugs inside the trusted boundary, faulty trusted arithmetic, adaptive corruption, and rollback without a trusted monotonic service or an erase-and-rekey lifecycle are not modeled; \cref{sec:sec-boundary,sec:discussion} discuss them.

\textbf{What the modules learn.}
Under \ProfT a module may see plaintext values; for example, after a verified masked opening it knows both $c$ and $r$, hence $x$. This is not leakage to the adversary because $\mathcal{F}_{\mathsf{T}}$ is never corrupted, but it is a relocation of trust that the paper states openly. \ProfU (\cref{sec:threat-profileu}) removes the resource from the joint sampler and the MAC keys and is a separate backend.

\textbf{Composition within the protocol.}
The protocol invokes checked openings, epilogues and gate subprotocols under one ledger and one set of MAC keys. Rather than composing separately proven subprotocols, \cref{thm:main} is proved with a single simulator for the whole admitted execution (\cref{app:proof-main}), because the MAC keys and the hidden-key invariant of \cref{lem:hidden-key} are shared across all gates. The block-level results of \cref{app:proof-dpf,app:proof-auth,app:proof-gates} are the algebraic and distributional facts that this simulator uses.
