# Supplementary material for: Trusted Hardware Acceleration for Malicious-Secure Function Secret Sharing
Source: arXiv:2610.04818 source file (2026-10-03)
Supplement: Supplementary file 6 [file F_model.tex]

% ======================================================================
% Appendix F: analytical performance model behind every red number
% Owner of labels: app:model, tab:model-params
% ======================================================================
\section{Analytical Performance Model}
\label{app:model}

Every red number in this paper is produced by one deterministic analytical model, which we will release with the artifact. This appendix documents the model so that each estimate can be audited and later replaced by a measurement, one constant at a time. The model is deliberately simple: it is a calibration layer on top of the published semi-honest DFA results~\cite{dfa2026trusted}, not a substitute for the three experiments of \cref{sec:arch-deploy} (A100 software, ZCU102 prototype, Accel-Sim on-die study), none of which has passed its completion gate yet (\cref{sec:eval-method}). Numbers copied from DFA are black and cited; protocol and design constants are black; everything the model computes or assumes is red. The executed CPU reference tests (\cref{sec:eval-attack}) are not model outputs.

\begin{table*}[t]
\centering
\caption{Parameters of the analytical performance model. (a) Platform, design and malicious-security constants; black entries come from the DFA paper~\cite{dfa2026trusted}, the protocol, or the design, and red entries are estimates to be replaced by measurements. (b) Per-model calibration of the semi-honest trusted-DFA rows (all estimates); the last four rows compare the calibrated model with the published DFA latencies.}
\label{tab:model-params}
\footnotesize
\begin{minipage}[t]{0.555\textwidth}
\centering
\textbf{(a)} Constants\\[2pt]
\setlength{\tabcolsep}{3pt}
\begin{tabular}{l l p{0.43\linewidth}}
\hline
\textbf{Symbol} & \textbf{Value} & \textbf{Meaning (source)} \\
\hline
$\mathit{BW}_{\mathrm{L}}$, $\mathit{RTT}_{\mathrm{L}}$ & 1\,GB/s, 0.05\,ms & LAN, as in DFA~\cite{dfa2026trusted} \\
$\mathit{BW}_{\mathrm{W}}$, $\mathit{RTT}_{\mathrm{W}}$ & 70\,MB/s, 70\,ms & WAN, as in DFA~\cite{dfa2026trusted} \\
$f_{28}$, $f_{7}$ & 720, 910\,MHz & DFA clock at 28/7\,nm~\cite{dfa2026trusted} \\
$N_{\mathrm{AES}}$ & 64 & 16 DPF units $\times$ 4 AES~\cite{dfa2026trusted} \\
$\mathit{BW}_{\mathrm{NoC}}$ & 290\,GB/s & on-die DFA bandwidth~\cite{dfa2026trusted} \\
$N_{\mathrm{FUA}}$ & 128 & Mersenne-61 MAC lanes (design) \\
$t$; $\phi_{\mathrm{R}}$ & 3; 2 & MAC lanes; rounds per checked layer \\
$a_{\mathrm{chk}}$, $m_{\mathrm{chk}}$ & 3.5, 6 & AES blocks, field mults per checked element \\
\hline
$\mathit{BW}_{\mathrm{PCIe}}$ & \est{25\,GB/s} & staged host-to-GPU copy \\
$\mathit{BW}_{\mathrm{rr}}$ & \est{32\,GB/s} & material reread without GaC \\
$\mu_{\mathrm{M}}$ & \est{1.25} & exact Mersenne vs.\ $\Z_{2^{64}}$ GEMM \\
$\phi_{\mathrm{oth}}$, $\phi_{\mathrm{D}}$ & \est{1.35}, \est{1.45} & other GPU work; module FSS work \\
$\phi_{\mathrm{B}}$, $\phi_{\mathrm{cg}}$ & \est{1.30}, \est{1.30} & online bytes; CPU-GPU bytes \\
$\eta_{\mathrm{trip}}$, $\eta_{\mathrm{NoC}}$ & \est{0.10}, \est{0.30} & exposed (non-overlapped) fraction \\
$\phi_{\mathrm{mat}}$ & \est{1.9} & authenticated material without GaC \\
$P_{\mathrm{mod}}$ & \est{1.14\,W} & one module at 7\,nm (\cref{tab:hwcost}) \\
$\eta_{\mathrm{pipe}}$ & \est{0.85} (\est{0.90} SH) & DPF pipeline efficiency \\
$\kappa_{\mathrm{key}}$, $\kappa_{\mathrm{ev}}$, $\kappa_{\mathrm{E}}$ & \est{2.2}, \est{2.0}, \est{2.4} & dealer-based malicious baseline \\
$\eta_{\mathrm{PIR}}$, $P_{\mathrm{PIR}}$ & \est{0.93}, \est{188\,W} & \sys PIR vs.\ DFA; average power \\
$\kappa_{\mathrm{APIR}}$, $P_{\mathrm{GPU}}$ & \est{0.45}, \est{350\,W} & authenticated GPU-DPF PIR \\
\hline
\end{tabular}
\end{minipage}\hfill
\begin{minipage}[t]{0.43\textwidth}
\centering
\textbf{(b)} Per-model calibration\\[2pt]
\setlength{\tabcolsep}{3pt}
\begin{tabular}{l c c c c}
\hline
 & \textbf{ResNet} & \textbf{BERT} & \textbf{GPT-Neo} & \textbf{LLaMA} \\
\hline
$G_{\mathrm{lin}}$ (s) & \est{0.22} & \est{0.52} & \est{3.10} & \est{10.40} \\
$G_{\mathrm{oth}}$ (s) & \est{0.15} & \est{0.25} & \est{1.20} & \est{3.30} \\
$D$ (s) & \est{0.04} & \est{0.09} & \est{0.35} & \est{0.90} \\
$B_{\mathrm{on}}$ (GB) & \est{0.30} & \est{0.43} & \est{1.05} & \est{2.80} \\
$R$ & \est{190} & \est{561} & \est{1160} & \est{1970} \\
$k$ (J/s) & \est{29.0} & \est{21.2} & \est{24.5} & \est{20.8} \\
$W_{\mathrm{MAC}}$ (G) & \est{4.1} & \est{11.2} & \est{168} & \est{836} \\
$M_{\mathrm{NoC}}$ (M) & \est{38} & \est{52} & \est{310} & \est{1040} \\
$M_{\mathrm{open}}$ (M) & \est{12} & \est{25} & \est{140} & \est{520} \\
$M_{\mathrm{gate}}$ (M) & \est{9.0} & \est{20.0} & \est{95.0} & \est{330} \\
$t^{\mathrm{GPU}}_{\mathrm{FSS}}$ (s) & \est{0.34} & \est{0.49} & \est{1.85} & \est{6.90} \\
\hline
LAN, model & \est{0.73} & \est{1.42} & \est{5.93} & \est{18.01} \\
LAN, DFA & 0.73 & 1.42 & 5.93 & 18.0 \\
WAN, model & \est{18.0} & \est{46.4} & \est{101.0} & \est{193.0} \\
WAN, DFA & 18.0 & 46.4 & 101 & 193 \\
\hline
\end{tabular}
\end{minipage}
\end{table*}

% ======================================================================
\subsection{Structure of the Model}

\textbf{Additive critical path.}
For one inference query, the model writes the end-to-end latency on a network with bandwidth $\mathit{BW}$ and round-trip time $\mathit{RTT}$ as the sum of the compute terms on the critical path, the online bytes of one party divided by the bandwidth, and the number of dependent online rounds times the round-trip time:
\begin{equation*}
T(\mathit{BW},\mathit{RTT})=\sum_{c}T_c+\frac{B_{\mathrm{on}}}{\mathit{BW}}+R\cdot\mathit{RTT}.
\end{equation*}
Overlap between components is modeled only where it is explicit, through the exposed fractions $\eta$ of \cref{tab:model-params}. The two parties are symmetric, the query is processed alone (batch size one), and the host is assumed to schedule honestly; a malicious host can always slow the protocol down or abort it, which the security theorem permits and the model does not price.

\textbf{Peak engine rates.}
With one block per engine per cycle, the $N_{\mathrm{AES}}=64$ engines deliver $64\times720\,\text{MHz}=46.08$\,G blocks/s at 28\,nm and $58.24$\,G blocks/s at 7\,nm, and the field unit array delivers $N_{\mathrm{FUA}}f_7=128\times910\,\text{MHz}=116.48$\,G multiply-accumulates/s (92.16\,G at 28\,nm). These are peak design rates; sustained rates are obtained by the efficiency factors below.

% ======================================================================
\subsection{Calibration against the Semi-Honest DFA Rows}

The semi-honest trusted-DFA latencies of DFA~\cite{dfa2026trusted} are decomposed as
\begin{gather*}
T^{\mathrm{SH}}=G_{\mathrm{lin}}+G_{\mathrm{oth}}+D+X+\frac{B_{\mathrm{on}}}{\mathit{BW}}+R\cdot\mathit{RTT},\\
X=V_{\mathrm{cg}}/\mathit{BW}_{\mathrm{PCIe}},
\end{gather*}
where $G_{\mathrm{lin}}$ is GPU time for linear algebra over $\Z_{2^{64}}$, $G_{\mathrm{oth}}$ other GPU time, $D$ the DFA-side FSS time, $V_{\mathrm{cg}}$ the CPU-to-GPU volume printed by DFA (e.g., 2.55\,GB for BERT-Base~\cite{dfa2026trusted}), $B_{\mathrm{on}}$ the online bytes per party and $R$ the dependent online rounds. \Cref{tab:model-params}(b) lists the chosen values. With them, the model reproduces every trusted-DFA LAN and WAN latency to the precision that DFA prints; the largest relative deviation is \est{0.43\%}, for the ResNet-50 LAN entry (\est{0.733}\,s against the printed 0.73\,s).

We state plainly what this calibration does and does not establish. The two published latencies per model constrain only the compute sum $G_{\mathrm{lin}}+G_{\mathrm{oth}}+D$ and one linear combination of $B_{\mathrm{on}}$ and $R$. The five parameters are therefore not identifiable from DFA's tables alone. We fixed them under three constraints: the LAN and WAN rows are reproduced; $D$ is small relative to GPU time, consistent with DFA's observation that FSS evaluation is not the single-path bottleneck once keys no longer move~\cite{dfa2026trusted}; and $R$ is of the order of the nonlinear depth of the compiled networks~\cite{gupta2023sigma,jawalkar2024orca}. The split matters for the malicious estimates because the malicious factors act differently on each term, so profiling $G_{\mathrm{lin}}$, $G_{\mathrm{oth}}$, $B_{\mathrm{on}}$ and $R$ on the A100 baseline is the first step of the replacement plan at the end of this appendix. The GPU-only FSS evaluation time used by the dealer baseline is $t^{\mathrm{GPU}}_{\mathrm{FSS}}=D+(T^{\mathrm{GPU}}_{\mathrm{LAN}}-T^{\mathrm{UDFA}}_{\mathrm{LAN}})$, i.e., the calibrated DFA time plus the LAN gap between DFA's GPU and untrusted-DFA rows (for BERT-Base, \est{0.09}\,s plus $18.8-18.4$\,s~\cite{dfa2026trusted}).

For energy, the model uses a per-model constant $k=E^{\mathrm{SH}}/(G_{\mathrm{lin}}+G_{\mathrm{oth}}+D)$, the published trusted-DFA energy~\cite{dfa2026trusted} divided by the calibrated compute time (e.g., $18.2\,\text{J}/\est{0.86}\,\text{s}=\est{21.2}$\,J/s for BERT-Base). $k$ is a calibration constant that inherits DFA's energy accounting; it is not a measured power draw.

% ======================================================================
\subsection{Malicious-Security Transformation}

\textbf{Authenticated linear algebra.}
Every linear layer runs on the GPU as $1+t$ exact-field GEMMs of the same shape: the value lane and one lane per MAC key, stored as separate coalesced arrays. Each lane uses the exact Mersenne reduction of \cref{sec:arch-field}, whose extra high-word multiply and two folds cost a factor $\mu_{\mathrm{M}}$ over wraparound $\Z_{2^{64}}$ arithmetic:
\begin{gather*}
G'_{\mathrm{lin}}=(1+t)\,\mu_{\mathrm{M}}\,G_{\mathrm{lin}},\\
G'_{\mathrm{oth}}=\phi_{\mathrm{oth}}G_{\mathrm{oth}},\qquad D'=\phi_{\mathrm{D}}D .
\end{gather*}
The factor $1+t=4$ is structural; $\mu_{\mathrm{M}}$, $\phi_{\mathrm{oth}}$ and $\phi_{\mathrm{D}}$ are estimates. $\phi_{\mathrm{D}}$ covers the malicious generate-and-consume (both generator states plus the evaluator), the output conversion into $\Fp$, the epilogue, and the compiler's gate mix. For BERT-Base, $G'_{\mathrm{lin}}=4\times\est{1.25}\times\est{0.52}=\est{2.60}$\,s.

\textbf{Communication and rounds.}
Canonical 64-bit field words, residuals and certificates enlarge online bytes and host-to-GPU volume, $B'_{\mathrm{on}}=\phi_{\mathrm{B}}B_{\mathrm{on}}$ and $V'_{\mathrm{cg}}=\phi_{\mathrm{cg}}V_{\mathrm{cg}}$. Every checked layer exchanges frozen value shares and then residuals (\cref{alg:checkopen}), so $R'=\phi_{\mathrm{R}}R=2R$. Offline communication is zero because all correlations are generated inside the modules.

\textbf{Triple generation.}
Each module generates the matrix triples jointly with its peer inside the protected boundary, one multiply-accumulate per linear-layer MAC, on the field unit array: $T_{\mathrm{trip}}=W_{\mathrm{MAC}}/(N_{\mathrm{FUA}}f_7)$. Generation for layer $\ell+1$ overlaps GPU work on layer $\ell$, so only $\eta_{\mathrm{trip}}T_{\mathrm{trip}}$ is exposed when $T_{\mathrm{trip}}<G'_{\mathrm{lin}}$, and $(T_{\mathrm{trip}}-G'_{\mathrm{lin}})+\eta_{\mathrm{trip}}G'_{\mathrm{lin}}$ otherwise. For LLaMA2-7B, $T_{\mathrm{trip}}=\est{836}\,\text{G}/116.48\,\text{G/s}=\est{7.18}$\,s per module, of which \est{0.72}\,s is exposed behind \est{52.0}\,s of authenticated GEMM.

\textbf{Module traffic and checks.}
Authenticated tuples cross the module boundary at 32 bytes per element per party, $V_{\mathrm{NoC}}=32M_{\mathrm{NoC}}$ (\est{1.66}\,GB per party for BERT-Base), and the exposed transfer time is $\eta_{\mathrm{NoC}}\cdot 2V_{\mathrm{NoC}}/\mathit{BW}_{\mathrm{link}}$ with $\mathit{BW}_{\mathrm{link}}=\mathit{BW}_{\mathrm{NoC}}$ on die. For an external module, each of the $R$ checked layers additionally pays two device round trips of \est{4}\,$\mu$s. The check engine spends $a_{\mathrm{chk}}=3.5$ AES blocks per checked element ($t/2=1.5$ blocks of challenge derivation, since one 128-bit block yields two 61-bit candidates, plus 2 blocks to AEAD-freeze a 32-byte tuple) and $m_{\mathrm{chk}}=2t=6$ field multiplications for the residuals, giving $T_{\mathrm{chk}}=M_{\mathrm{open}}\bigl(a_{\mathrm{chk}}/(N_{\mathrm{AES}}f_7)+m_{\mathrm{chk}}/(N_{\mathrm{FUA}}f_7)\bigr)$.

\textbf{Total and energy.}
The malicious latency is
\begin{align*}
T^{\mathrm{Mal}}={}&G'_{\mathrm{lin}}+G'_{\mathrm{oth}}+D'+X'+T^{\mathrm{exp}}_{\mathrm{trip}}+T^{\mathrm{exp}}_{\mathrm{NoC}}\\
&+T_{\mathrm{chk}}+B'_{\mathrm{on}}/\mathit{BW}+2R\cdot\mathit{RTT},
\end{align*}
with $X'=V'_{\mathrm{cg}}/\mathit{BW}_{\mathrm{PCIe}}$,
and the energy is $E^{\mathrm{Mal}}=k\,(G'_{\mathrm{lin}}+G'_{\mathrm{oth}}+D')+2P_{\mathrm{mod}}T^{\mathrm{Mal}}_{\mathrm{LAN}}$, i.e., calibrated GPU-side energy plus two modules powered for the whole query. For BERT-Base on LAN the terms are \est{2.60}\,s (authenticated GEMM), \est{0.338}\,s (other GPU), \est{0.131}\,s (module FSS), \est{0.133}\,s (host-to-GPU copy), \est{0.010}\,s (exposed triples), \est{0.003}\,s (module traffic), \est{0.003}\,s (checks) and \est{0.615}\,s (network), for a total of \est{3.83}\,s, of which authenticated GEMM is \est{68\%}. The energy is $\est{64.9}+\est{8.7}=\est{73.7}$\,J. These are the \sys rows of \cref{tab:e2e} and the breakdown of \cref{fig:bert}.

\textbf{Without generate-and-consume.}
The ablation that materializes authenticated FSS material stores and rereads $\phi_{\mathrm{mat}}$ times DFA's no-GaC CPU-to-GPU volume~\cite{dfa2026trusted} and pays $(\phi_{\mathrm{mat}}V^{\mathrm{noGaC}}_{\mathrm{cg}}-V'_{\mathrm{cg}})/\mathit{BW}_{\mathrm{rr}}$ extra, with energy scaled by \est{1.05}. For BERT-Base this is $\est{1.9}\times 36.1$\,GB $=\est{68.6}$\,GB and \est{5.87}\,s on LAN.

% ======================================================================
\subsection{Baselines}

\textbf{Dealer-based malicious FSS.}
This baseline models an actively secure FSS protocol in the style of Shark~\cite{gupta2025shark}, with an external dealer that ships authenticated keys and preprocessing. It is \emph{not} a measurement of Shark: until a matching artifact is run, we make no performance claim relative to Shark itself. The model scales DFA's semi-honest GPU row~\cite{dfa2026trusted}: offline bytes and host-to-GPU volume grow by $\kappa_{\mathrm{key}}$ for authenticated keys and MAC material, GPU evaluation of authenticated keys takes $\kappa_{\mathrm{ev}}t^{\mathrm{GPU}}_{\mathrm{FSS}}$, energy grows by $\kappa_{\mathrm{E}}$, and the linear algebra, online bytes and doubled rounds are the same as for \sys. The offline material is sent over the same network as the online traffic. For BERT-Base on LAN this gives \est{37.6}\,s of offline distribution, \est{1.70}\,s of key copies, \est{2.60}\,s of authenticated GEMM, \est{0.338}\,s of other GPU work, \est{0.98}\,s of FSS evaluation and \est{0.615}\,s of network, i.e., \est{43.9}\,s in total. The bandwidth sweep of \cref{sec:eval-e2e} changes only $\mathit{BW}$: at 0.1\,GB/s the baseline needs \est{387}\,s against \est{8.86}\,s for \sys (\est{43.7$\times$}), and at 10\,GB/s \est{9.49}\,s against \est{3.33}\,s (\est{2.9$\times$}). The advantage is thus driven by offline distribution and shrinks as bandwidth grows, which is the expected behavior and the reason the comparison must eventually be repeated with the real artifact.

\textbf{PIR baselines and the power cross-check.}
The GPU-DPF and GPU+DFA PIR rows are DFA's numbers~\cite{dfa2026trusted}, read as queries/s and mJ/query. Multiplying throughput by energy per query yields an average power that must be physically plausible: $134\text{k}\times 2.61\,\text{mJ}\approx 350$\,W for GPU-DPF and $1125\text{k}\times 0.187\,\text{mJ}\approx 210$\,W for GPU+DFA at 16K entries, and the same two values within 2\,W at 1M and 4M entries. This cross-check is why \cref{tab:pir} reports mJ/query together with the implied power. \sys PIR is modeled as $\eta_{\mathrm{PIR}}$ times the DFA throughput, where the loss covers the snapshot hash of the consumed bytes, the fresh resharing and certificate generation, and lockstep batching, at an average power $P_{\mathrm{PIR}}$. $P_{\mathrm{PIR}}$ is below DFA's implied power because \cref{alg:pir} moves the DPF-weighted record reduction from the GPU into the protected field unit array; this is the least certain PIR parameter and the first to be measured. As a capacity sanity check, at 16K entries \sys evaluates \est{$1.05$\,M} queries/s $\times$ $2^{14}$ leaves $=\est{17.1}$\,G leaves/s; with 128-bit records split into three 61-bit coordinates, the reduction needs \est{51}\,G multiply-accumulates/s, below the 116.48\,G/s of the array. The authenticated GPU-DPF baseline in the style of APIR~\cite{colombo2023apir} is modeled as $\kappa_{\mathrm{APIR}}$ times GPU-DPF throughput at $P_{\mathrm{GPU}}$.

% ======================================================================
\subsection{Microbenchmark Models}

\textbf{Single-path DPF gates.}
A malicious generate-and-consume gate of depth $n$ performs $3n$ PRG expansions per module ($2n$ for the two generator states and $n$ for the evaluator), i.e., $6n$ AES blocks, plus \est{3} blocks for output conversion and pads. Its sustained throughput is $\eta_{\mathrm{pipe}}N_{\mathrm{AES}}f_{28}/(6n+3)$, versus $6n+1$ blocks for the semi-honest trusted DFA and $(1+t)6n+3$ for a design that authenticates outputs with one tag tree per lane. For $n=61$ this yields \est{106}, \est{113} and \est{26.7}\,M gates/s (\cref{fig:dpfthr}). The latency of one dependent gate is $(20n+\est{12})/f_{28}$, where 20 cycles per level is DFA's pipeline depth~\cite{dfa2026trusted}, i.e., \est{1.71}\,$\mu$s for $n=61$.

\textbf{Nonlinear gates.}
A width-$w$ LUT costs $2(2w+2^w-1)$ AES blocks (two-state generation along the target path plus full-domain evaluation) and $2^w+w+4$ field multiplications; the conservative interval gate costs two DCFs of $n(n+1)/2$ path levels at 6 blocks per level, $2\cdot 6\cdot n(n+1)/2=22692$ blocks for $n=61$; the projected optimized interval gate assumes \est{8} blocks per level for two $O(n)$ DCFs (\est{976} blocks) and is not covered by \cref{thm:dcf}. Bit decomposition costs $2n$ multiplications in $2n+1$ rounds, and exact truncation $5n+2$ multiplications (\cref{app:proof-gates}). The LAN latency of a gate is its round count times $2\mathit{RTT}$ (value exchange and residual exchange) plus its AES and multiplication time at peak rates. The model charges the LUT and interval gates a single checked round, assuming their bit-level products are batched with the preceding layer's openings. These are the entries of \cref{tab:gates}.

\textbf{\CheckOpen.}
For a batch of $m$ elements, the latency is the sum of freezing at \est{100}\,GB/s plus \est{0.2}\,$\mu$s, the value exchange ($8m/\mathit{BW}+\mathit{RTT}$), challenge derivation ($mt/2$ AES blocks), residual computation ($2mt$ multiplications), the residual exchange ($8t/\mathit{BW}+\mathit{RTT}$), and a fixed \est{0.5}\,$\mu$s for the decision. On LAN with $t=3$ this is \est{0.101}\,ms for $m=64$ and \est{0.652}\,ms (\est{100}\,M elements/s) for $m=65536$; the two round trips dominate small batches and $t$ barely matters (\cref{fig:checkperf}).

\textbf{Ablations and sweeps.}
Each ablation of \cref{tab:ablation} changes one input of the model: tag trees replace the epilogue by scaling $D'$ by $(1+t)$ times an overlap factor \est{0.8}; $t=1,2$ change the lane count; FSS-only configurations set $D'=M_{\mathrm{gate}}/\text{throughput}$ of the respective interval gate; direct-only scales $D$ by \est{1.30}; small batches add \est{0.41}\,s of per-batch overhead; the external PCIe module sets $\mathit{BW}_{\mathrm{link}}=\est{25}$\,GB/s with per-round device trips; the ZCU102 configuration sets $\mathit{BW}_{\mathrm{link}}=\est{1.6}$\,GB/s and a triple rate of \est{32} lanes at \est{250}\,MHz (\cref{tab:fpga}); and the no-check configuration keeps $R'=R$, which is an insecure lower bound rather than a secure variant.

% ======================================================================
\subsection{Validity Limits and Replacement Plan}

\textbf{Known blind spots.}
The model ignores contention between tag-lane GEMMs and module traffic beyond the exposed fraction $\eta_{\mathrm{NoC}}$, assumes that the compiler batches independent checks perfectly, uses peak engine rates scaled by constant efficiencies, and does not model network jitter, queueing, or the cost of an adversarial host scheduler. Its outputs are therefore planning estimates; the security statements of \cref{sec:security} do not depend on any of them, and no security parameter is ever inferred from a measurement.

\textbf{Replacement plan.}
Each red value traces to the constants of \cref{tab:model-params}, and each constant has a designated measurement.
\begin{enumerate}[leftmargin=*,label=(\roman*)]
\item \emph{A100 software} (\cref{sec:arch-deploy}): profile the Sigma and Orca baselines~\cite{gupta2023sigma,jawalkar2024orca} to replace the calibration of \cref{tab:model-params}(b), and time the exact field kernels on four lanes to replace $\mu_{\mathrm{M}}$, $\phi_{\mathrm{oth}}$, $\mathit{BW}_{\mathrm{PCIe}}$ and $\mathit{BW}_{\mathrm{rr}}$.
\item \emph{ZCU102 prototype}~\cite{amd2023zcu102}: measure the DPF pipeline efficiency, the field unit array, the check engine and AEAD freeze throughput, and the host link, which replaces $\eta_{\mathrm{pipe}}$, the triple rate, the \CheckOpen{} constants and the external-link rows; board energy comes from rail or wall power, distinct from tool estimates.
\item \emph{Accel-Sim on-die study}~\cite{khairy2020accel}: simulate module traffic next to L2, as DFA did, to replace $\eta_{\mathrm{NoC}}$, $\eta_{\mathrm{trip}}$, $\eta_{\mathrm{PIR}}$ and $P_{\mathrm{PIR}}$.
\item \emph{Synthesis}: 28\,nm synthesis of the new blocks with DeepScaleTool scaling~\cite{sarangi2021deepscaletool} replaces $P_{\mathrm{mod}}$ and the hardware-cost tables.
\item \emph{Baseline artifacts}: running an actively secure FSS artifact~\cite{gupta2025shark} and an authenticated PIR artifact~\cite{colombo2023apir} replaces $\kappa_{\mathrm{key}}$, $\kappa_{\mathrm{ev}}$, $\kappa_{\mathrm{E}}$ and $\kappa_{\mathrm{APIR}}$.
\end{enumerate}
All measurements follow the protocol of \cref{sec:eval-method}: 5 warm-up and 30 measured repetitions, median and 95th percentile with bootstrap confidence intervals, raw per-run records, GPU energy as the integral of sampled power over the measurement window, and the power cross-check above for every energy-per-query figure. The three experiments remain separate; their timings are never merged into a single number presented as fully measured.
