# Supplementary material for: Trusted Hardware Acceleration for Malicious-Secure Function Secret Sharing
Source: arXiv:2610.04818 source file (2026-10-03)
Supplement: Supplementary file 29 [file harness_r2_appendix_E_proofs_main_tex.tex]

\documentclass[journal]{IEEEtran}
\input{../macros}
\renewcommand{\includegraphics}[2][]{\fbox{\detokenize{#2}}}
\begin{document}
\appendices
\input{../appendix/E_proofs_main}
\end{document}
